# Supplementary material for: Strength of minority ties: the role of homophily and group composition in a weighted social network
Source: arXiv:2311.06384 source file (2024-01-27)
Supplement: Supplementary file 1 [file supplement.pdf]

# Supplementary material for:
# Strength of minority ties: the role of homophily and group composition in a weighted social network

J. R. Nicolás-Carlock*[1], D. Boyer[1], S. E. Smith-Aguilar[2], and G. Ramos-Fernández[2]

[1]Instituto de Física, Universidad Nacional Autónoma de México, México
[2]Instituto de Investigaciones en Matemáticas Aplicadas y en Sistemas, Universidad Nacional Autónoma de México, México

*Correspondence: jnicolas@unam.mx

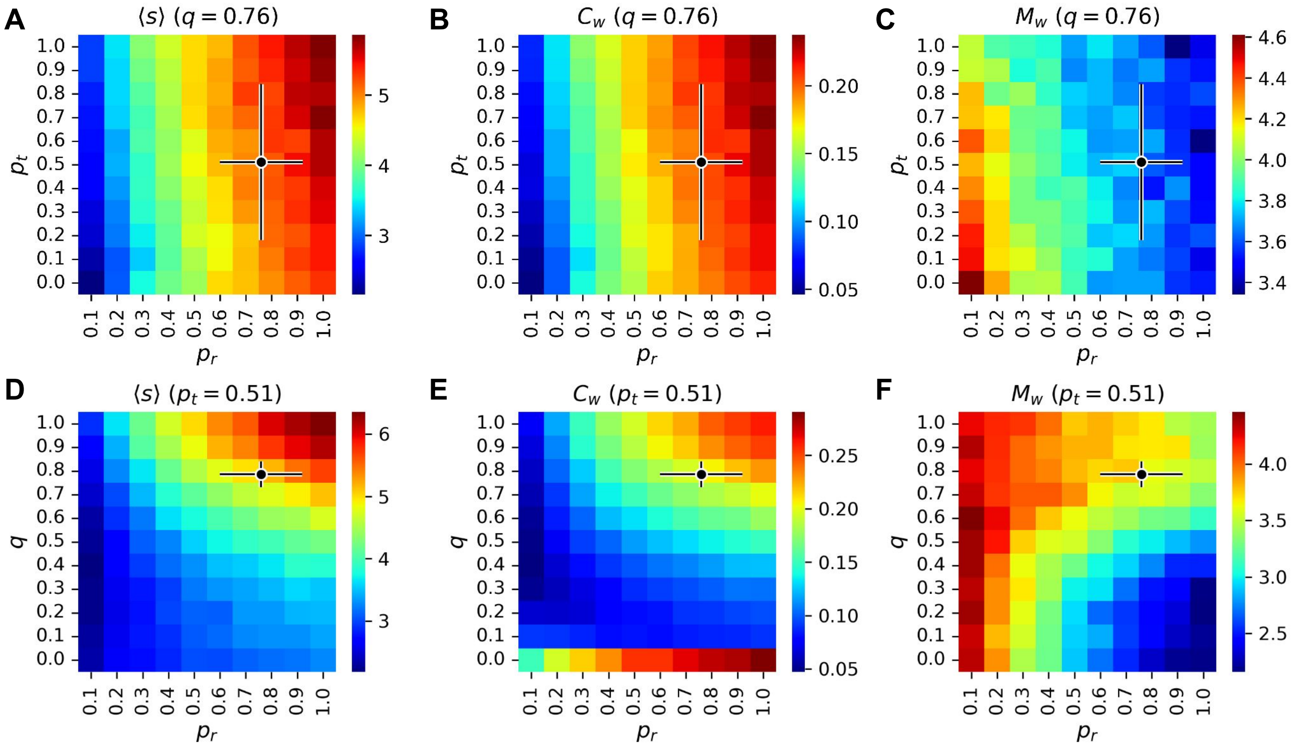


Figure S1: **Weighted metrics in parameter space.** (A)-(F) The heatmaps represent slices in parameter space $(p_r, q_t, q)$ of the average weighted metrics produced by the extended WSN model. Slices correspond to the values in the parenthesis on top. The colors are proportional to the corresponding metric values. The dot and crossed bars indicate the average and standard deviations of the parameters' distributions in Fig. 3b, of the association network A+SA+J, with $(p_r, p_t, q) = (0.7, 0.5, 0.7)$.

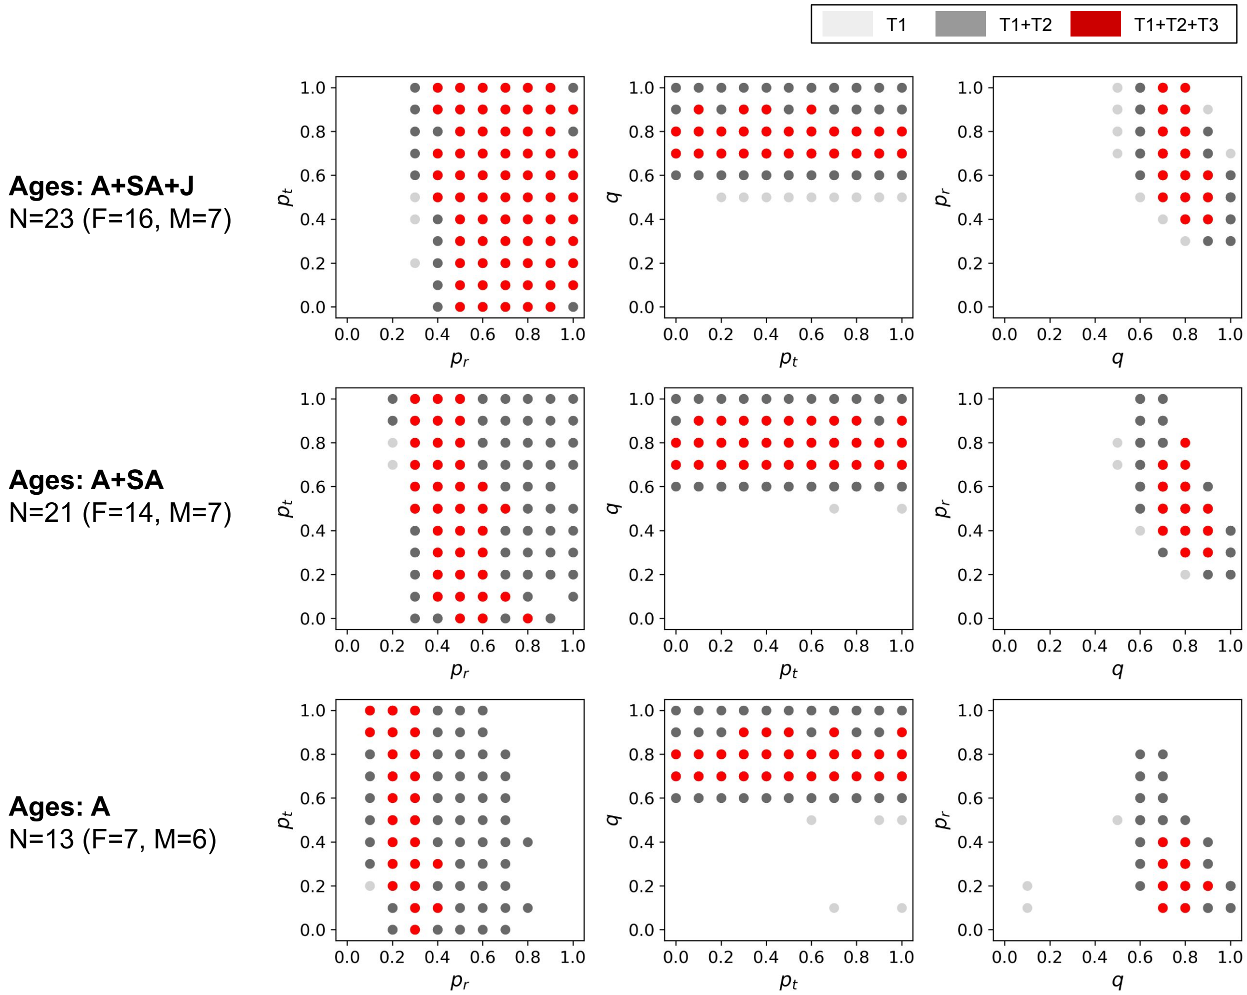


Figure S2: **Parameters distributions for different ages.** Distribution of points in parameter space that pass the significance test, as indicated by the color key on top, for the network with A+SA+J (top row), A+SA (middle row), and just A (bottom row). The parameters used were: A+SA+J, with $(p_r, p_t, q) = (0.7, 0.5, 0.7)$; A and SA, with $(p_r, p_t, q) = (0.5, 0.5, 0.8)$, A, with $(p_r, p_t, q) = (0.2, 0.5, 0.8)$.

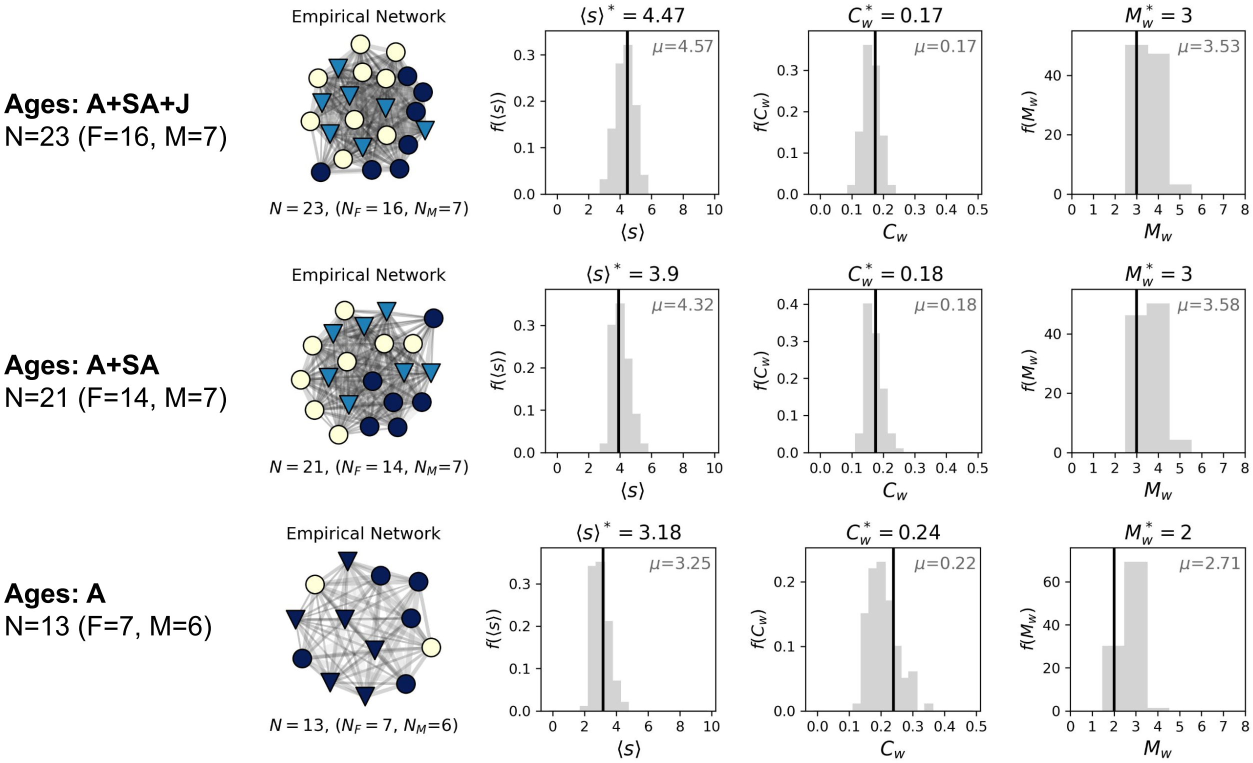


Figure S3: **Results on different age categories: weighted macro properties.** Results of the two-tailed significance test ($\alpha = 0.05$) based on the weighted metrics for the association networks with A+SA+J (top row), A+SA (middle row), and A (bottom row). Each distribution is generated using the average values, $(\langle p_r \rangle, \langle q_t \rangle, \langle q \rangle)$, indicated in Fig. 3b, 3d, and 3f in the main text. Empirical metrics are indicated with an asterisk (*) on top of the plots. A visualization of the corresponding empirical association network is also shown with node colors indicated the node's module. The parameters used were: A+SA+J, with $(p_r, p_t, q) = (0.7, 0.5, 0.7)$; A and SA, with $(p_r, p_t, q) = (0.5, 0.5, 0.8)$, A, with $(p_r, p_t, q) = (0.2, 0.5, 0.8)$.

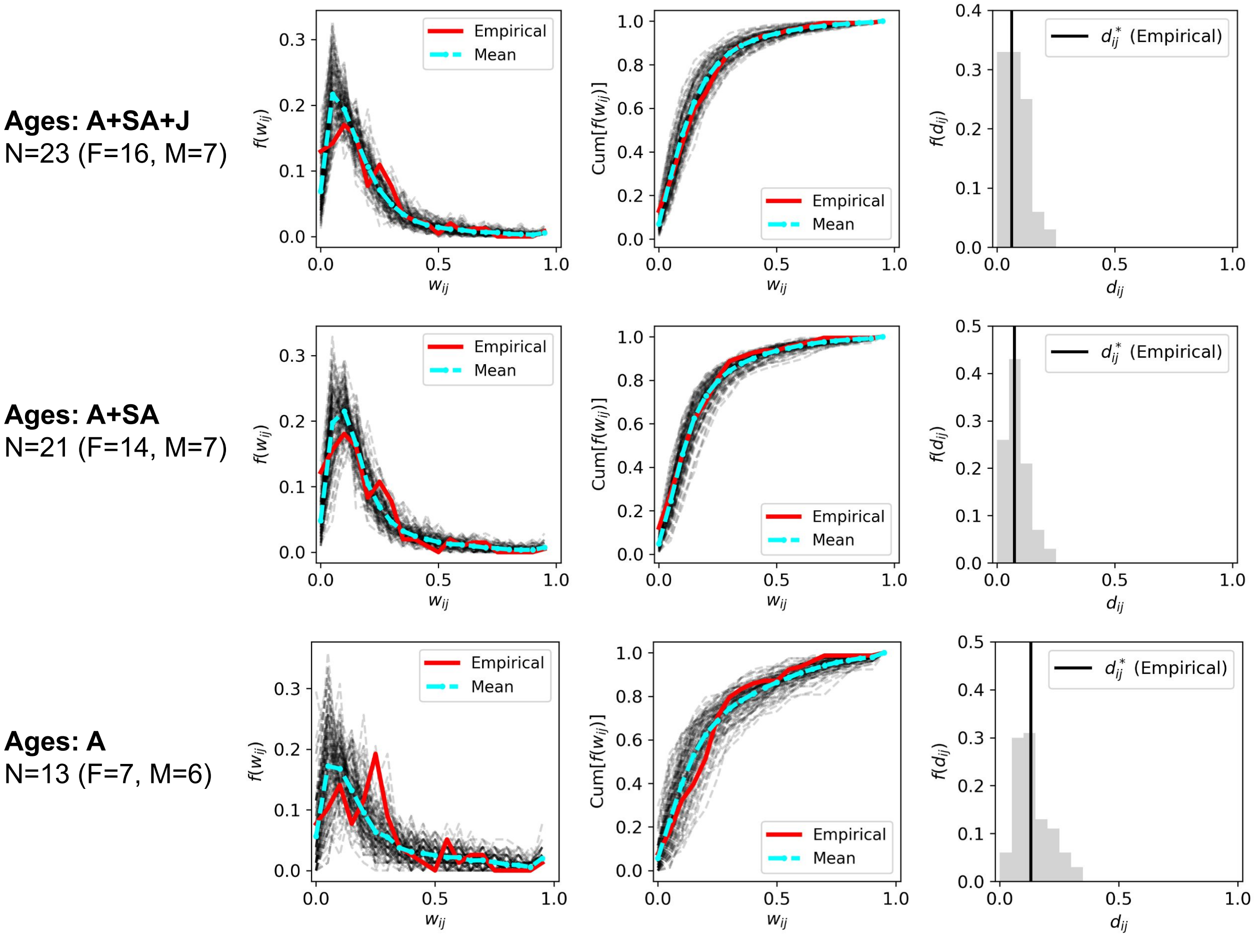


Figure S4: **Results on different age categories: weight distribution.** Results of the single-tailed significance test ($\alpha = 0.10$) based on the Kolmogorov-Smirnov distance for the association networks with A+SA+J (top row), A+SA (middle row), and A (bottom row). Each distribution is generated using the average values, $(\langle p_r \rangle, \langle q_t \rangle, \langle q \rangle)$, indicated in Fig. 3b, 3d, and 3f, in the main text. Empirical and numerical mean distributions are indicated. The parameters used were: A+SA+J, with $(p_r, p_t, q) = (0.7, 0.5, 0.7)$; A and SA, with $(p_r, p_t, q) = (0.5, 0.5, 0.8)$, A, with $(p_r, p_t, q) = (0.2, 0.5, 0.8)$.

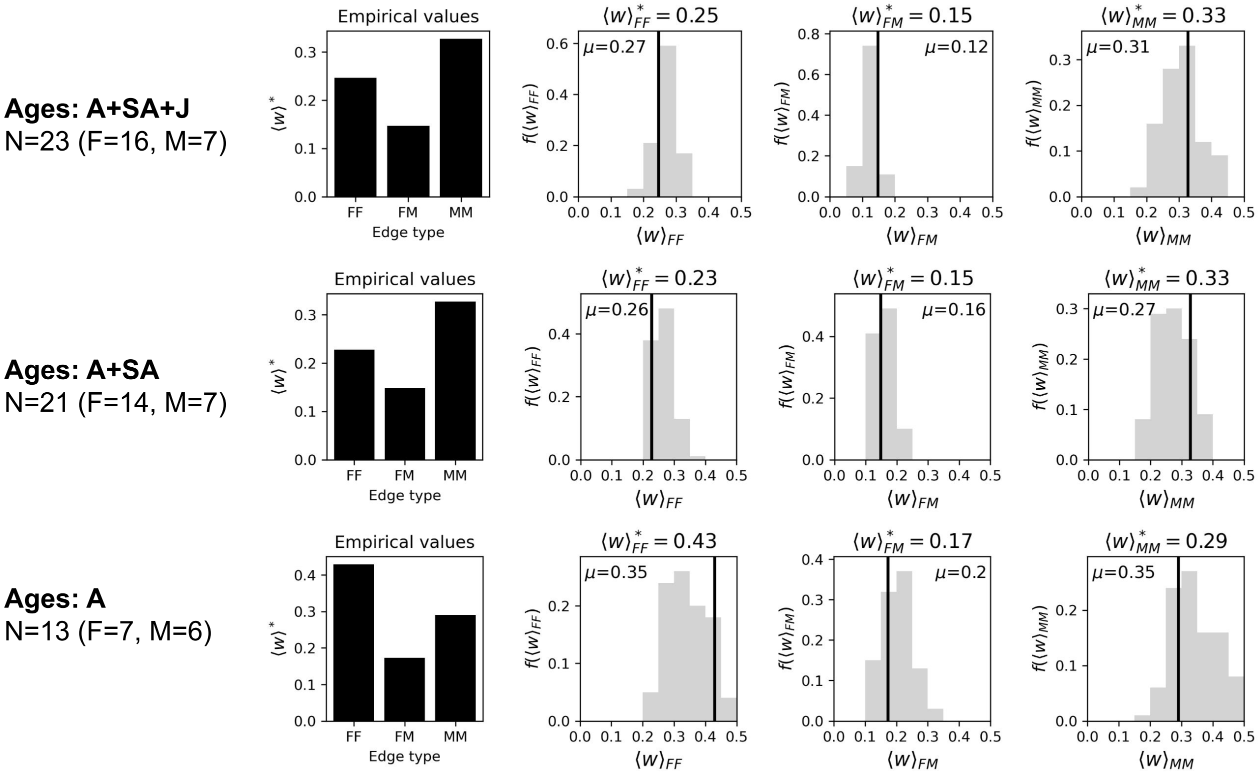


Figure S5: **Results on different age categories: average weight per edge-type.** Results of the two-tail significance test ($\alpha = 0.05$) based on the average weight per edge type for the association networks with A+SA+J (top row), A+SA (middle row), and A (bottom row). Each distribution is generated using the average values, $(\langle p_r \rangle, \langle q_t \rangle, \langle q \rangle)$, indicated in Fig. 3b, 3d, and 3f of the main text. Empirical metrics are indicated with an asterisk (*) on top of the plots. A bar plot (in black) of the corresponding empirical values is also shown. The parameters used were: A+SA+J, with $(p_r, p_t, q) = (0.7, 0.5, 0.7)$; A and SA, with $(p_r, p_t, q) = (0.5, 0.5, 0.8)$, A, with $(p_r, p_t, q) = (0.2, 0.5, 0.8)$.
